# Supplementary material for: Contractile units in disordered actomyosin bundles arise from F-actin buckling
Source: arXiv:1201.4110 ancillary file (2012-01-19)
Supplement: Supplementary file 1 [file SupplementalMaterial.pdf]

# Contractile units in disordered actomyosin bundles arise from F-actin buckling

## Supporting material

### EXPERIMENTAL METHODS

The preparation of reconstituted bundles comprised of filamentous actin (F-actin) and filaments of smooth muscle myosin motors is described in detail in Ref. [1]. All imaging is performed with a spinning disk confocal microscope with a 60 $\times$ , NA 1.2 lens. A dilute suspension of biotinylated polystyrene carboxylate beads coated with neutravidin in Wash Buffer (20 mM MOPS, pH 7.4, 50 mM KCl, 4 mM MgCl<sub>2</sub>, 0.1 mM EGTA) is perfused into a flow chamber loaded with a coverslip covered with a 10-20  $\mu$ m thick polyacrylamide gel onto which biotinylated bovine serum albumin (BSA) is covalently attached. The beads sediment and bind to the biotinylated BSA, and unbound beads are removed by perfusion of Wash Buffer.

F-actin stabilized with Alexa 568 phalloidin and containing 10% biotinylated G-actin is gently sheared to an average length  $\ell_f = 6 \mu$ m, diluted to 1  $\mu$ M in Assay Buffer (20 mM MOPS, pH 7.4, 100 mM KCl, 4 mM MgCl<sub>2</sub>, 0.1 mM EGTA, 0.7% methylcellulose, 0.25 mg  $\cdot$  ml<sup>-1</sup> glucose, 0.25%  $\beta$ -ME, 0.25 mg  $\cdot$  ml<sup>-1</sup> glucose oxidase, 0.25  $\mu$ g  $\cdot$  ml<sup>-1</sup> catalase) and loaded into the chamber. Over the course of 30 minutes, F-actin binds to avidin beads to form “asters” as shown in Fig. S1(a). Most of the unbound actin is then removed by perfusion of Assay Buffer. Oregon Green-labeled smooth muscle myosin thick filaments in Assay Buffer are then perfused into the chamber and bundles of lengths 10-100  $\mu$ m bound to the beads form over a period of 20 minutes [Fig. S1(b)]. All assembly steps are presumably independent on the polarity of F-actin, thus likely resulting in bundles with mixed polarities. Additionally, observation in fluorescence microscopy fails to reveal any spatial organization reminiscent of sarcomeres [1]. The density of myosin filaments within the bundle is tuned by varying the concentration of smooth muscle myosin from 0.1 to 1  $\mu$ M. By measuring the actin and myosin densities inside the bundle by quantitative fluorescence microscopy and SDS-PAGE, we establish that they correspond to an average distance  $\ell_0$  between myosin thick filaments along individual F-actin varying from 390 nm to 5.3  $\mu$ m [1].

After bundle formation, Assay Buffer containing 1 mM ATP is perfused into the imaging chamber to initiate bundle contraction [Fig. S1(c)]. To facilitate imaging, we only consider bundles bound to polystyrene beads at both ends in this work. The extent of bundle contraction is assessed by measuring the bundle contour length  $L_b$  prior to and after contraction. The relative bundle deformation

is defined as

$$\frac{L_b - L_b(\text{before contraction})}{L_b(\text{before contraction})}. \quad (\text{S1})$$

Bundles much longer than  $\ell_f$  contract with a velocity proportional to their lengths [1], indicating that contraction occurs throughout the bundle. This excludes the possibility that contraction is an end effect due to a hypothetical alignment of the filament polarities at the beads. Buckles present during contraction are quantified by visually detecting the number of F-actin extending from the bundle centerline during contraction on a frame by frame basis.

### REQUIREMENTS FOR NON-SARCOMERIC BUNDLE CONTRACTION

A key notion underlying the proposed mechanism for non-sarcomeric bundle contraction is the recognition that actin-myosin interactions can *a priori* elicit extension just as well as contraction. While this is illustrated in Fig. 1(c) of the main text in the case of two very simple bundles, here we present a more general discussion. In this section, we show that contractile behavior in the absence of sarcomeric organization requires

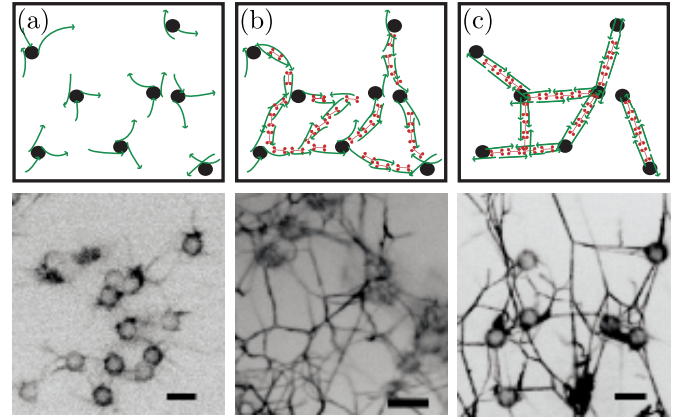

FIG. S1. Formation and contraction of reconstituted actomyosin bundles. *Top*: schematics. *Bottom*: corresponding inverted contrast confocal micrographs of fluorescent actin (a) and myosin (b-c). (a) Formation of actin asters following perfusion of biotinylated F-actin (*green*) into the flow chamber containing avidin-coated polystyrene beads (*black*). (b) Formation of bundles following perfusion of myosin thick filaments (*red*) in the absence of ATP. (c) Bundle contraction following the perfusion of ATP. Scale bars, 5  $\mu$ m

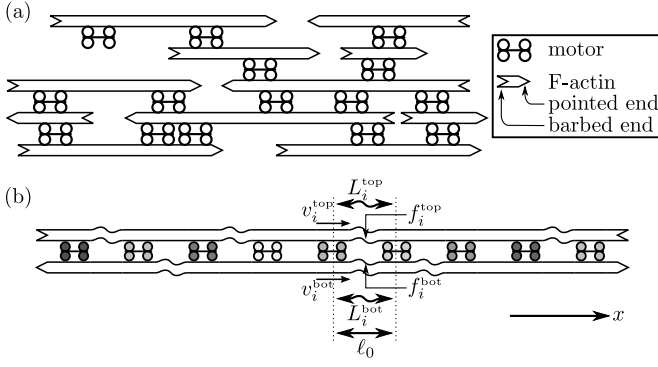

FIG. S2. Structures considered to establish the requirements for non-sarcomeric contractility. (a) Arbitrary bundle with identical motors, which does not lead to contractility. (b) Simplified bundle with two filaments and non-identical motors (shades of grey). This structure leads to contractility only if the filaments respond asymmetrically to compression and extension.

- (i) a dispersion in the velocities of the motors within the bundle;
- (ii) an asymmetric elastic response of the filaments to compressive and extensile stresses.

#### Dispersion of motor velocities (i)

To prove the necessity of condition (i), we consider a large bundle of arbitrary topology comprising only filaments aligned in the  $x$  direction and identical motors [Fig. S2(a)]. When bound to a filament and in the absence of load, a motor moves towards its barbed end (away from the pointed end) with a relative speed  $v$ . Due to the large number of myosin heads present within a single motor, each motor can be connected to one or more filaments. A motor reaching the end of a filament continues to move at velocity  $v$  relative to it until it detaches. Here we show by recursion that in this setting all motors are motionless relative to one another, while filaments with pointed ends facing right move relative to the motors with velocity  $+v$ , and filaments with pointed ends facing left move relative to the motors with velocity  $-v$ . We define this as the filament translation property (FTP). Further discussion of our assumptions as well as a slightly more general proof are presented in Ref. [2].

The FTP is manifestly true for the smallest possible bundle, which comprises just one motor and no filament. For convenience, we choose our reference frame such that the velocity of this first motor is equal to zero. Assuming that the FTP is valid for all  $n$ -bundles (*i.e.*, bundles with  $n$  motors or filaments), we increase the bundle size by one element through one of the three following operations:

1. Addition of a motor, which may be connected to

several filaments. Since the motor moves towards filament barbed ends with a relative speed  $v$ , its velocity relative to a right-pointing filament to which it is connected is  $-v$ . Since the FTP is assumed to hold true for the  $n$ -bundle, right-pointing filaments move with velocity  $+v$  and, thus, the motor's absolute velocity in our reference frame is 0. A similar argument holds in the case of contact with a left-pointing filament. Therefore contact with one or several filaments of arbitrary polarity consistently imposes a zero velocity on the motor, and the FTP is respected.

2. Addition of a right-pointing filament, which may be connected to several motors. Since motors have a velocity 0 and move towards F-actin barbed ends with a relative speed  $v$ , the filament's velocity relative to any motor to which it is connected is  $+v$  and, thus, its absolute velocity in our reference frame is  $+v$ . Thus, regardless of the number of motors connected to the filament, the FTP is respected.
3. Addition of a left-pointing filament—this case is the mirror image of case 2, with similar conclusions.

Since any  $(n+1)$ -bundle can be constructed by adding a motor or filament to some  $n$ -bundle, this implies that the FTP is true for all  $(n+1)$ -bundles and provides a complete proof of the FTP by recursion.

As a consequence of the FTP, motors function as conveyor belts which slide the right-pointing filaments to the right with velocity  $+v$ , and the left-pointing filaments to the left with velocity  $-v$ . Therefore, the relative velocity of the two ends of the bundle can only be  $-2v$ , 0, or  $+2v$  depending on the polarity of the filaments present. This means that contraction or extension of the bundle can only be an end effect, which does not support the well-defined contraction velocity per unit length observed in Refs. [1, 3–5]. This conclusion also applies to bundles where the motors are allowed to attach to and detach from the filaments, either stochastically or upon reaching the filament end. Indeed, a detachment or reattachment event can be viewed as a modification in the bundle topology. As the FTP applies to bundles with identical motors irrespective of their topology, it applies both before and after the attachment/detachment event. Thus, bundles comprised of filaments with identical motors are non-contractile, as previously observed in numerical simulations [6].

#### Asymmetric elastic response of the filaments (ii)

To demonstrate the necessity of condition (ii), we show that bundles where non-identical motors are present fail to contract in the absence of an asymmetric elastic response of their filaments to applied stresses. While we do

not present a general demonstration valid for arbitrary bundle topologies and nonlinear motor force-velocity relationships here, such a proof can be derived and is presented in the more technical Ref. [2].

Here we restrict our argument to the simple bundle presented in Fig. S2(b). Our specific goal is to show that no external force is required to keep motors immobile in the case where filaments respond symmetrically to elastic stresses. From this, we conclude that a symmetric elastic response of the filaments precludes contraction.

As in the main text, we subdivide the two filaments of length  $\ell_f$  into filament sections labeled by  $i = 0, \dots, N$  with  $N = \ell_f/\ell_0$ . We introduce the tensions  $f_i^{\text{top}}$  and  $f_i^{\text{bot}}$  of the  $i$ th sections of the top and bottom filaments, respectively. We also denote their contour lengths by  $L_i^{\text{top}}$  and  $L_i^{\text{bot}}$ . We consider an initially relaxed bundle with the  $i = 0$  and  $i = N$  ends of the filament dangling in solution. This imposes the conditions

$$f_i^{\text{top}}(t=0) = f_i^{\text{bot}}(t=0) = 0 \quad (\text{S2a})$$

$$L_i^{\text{top}}(t=0) = L_i^{\text{bot}}(t=0) = L_0 \quad (\text{S2b})$$

$$f_0^{\text{top}}(t) = f_N^{\text{top}}(t) = f_0^{\text{bot}}(t) = f_N^{\text{bot}}(t) = 0. \quad (\text{S2c})$$

We label the motor flanked by filament sections  $i-1$  and  $i$  as motor  $i$ , and denote the local velocity of the top (bottom) filament relative to motor  $i$  as  $v_i^{\text{top}}$  ( $v_i^{\text{bot}}$ ). A summary of these notations is presented in Fig. S2(b).

We assume that the motors are held fixed, and denote by  $\ell_0$  the distance between two consecutive motors. We introduce a set of forces  $\{f_i^{\text{ext}}\}_{i=1\dots N}$ , where  $f_i^{\text{ext}}$  is exerted from the outside on motor  $i$  to hold it in place. These forces can be seen as Lagrange multipliers conjugate to the motors' positions. The magnitude of  $f_i^{\text{ext}}$  can be calculated by expressing force balance on motor  $i$ :

$$f_i^{\text{ext}} = -f_i^{\text{top}} - f_i^{\text{bot}} + f_{i-1}^{\text{top}} + f_{i-1}^{\text{bot}}. \quad (\text{S3})$$

As discussed above, if all  $\{f_i^{\text{ext}}\}_{i=1\dots N}$  can be shown to vanish, then the bundle is non-contractile.

The dynamics of the bundle is described by equations that parallel Eqs. (1), (2) and (4) of the main text. We first write the filament force-extension relationships

$$L_i^{\text{top}} - L_0 = \mathcal{L}(f_i^{\text{top}}) \quad (\text{S4a})$$

$$L_i^{\text{bot}} - L_0 = \mathcal{L}(f_i^{\text{bot}}), \quad (\text{S4b})$$

where the full non-linear dependence of the filament extension on the force is described by the unspecified function  $\mathcal{L}$ . Next are the motor force-velocity relationships

$$f_{i-1}^{\text{top}} - f_i^{\text{top}} = F_i - \chi v_i^{\text{top}} \quad (\text{S5a})$$

$$f_{i-1}^{\text{bot}} - f_i^{\text{bot}} = -F_i - \chi v_i^{\text{bot}}, \quad (\text{S5b})$$

with  $\chi > 0$ . Finally, filament mass conservation gives

$$\frac{dL_i^{\text{top}}}{dt} = v_i^{\text{top}} - v_{i+1}^{\text{top}} \quad (\text{S6a})$$

$$\frac{dL_i^{\text{bot}}}{dt} = v_i^{\text{bot}} - v_{i+1}^{\text{bot}}. \quad (\text{S6b})$$

Combining Eqs. (S4-S6), we can write evolution equations for the bundle forces in a closed form:

$$\chi \frac{d\mathcal{L}(f_i^{\text{top}})}{dt} - (f_{i-1}^{\text{top}} - 2f_i^{\text{top}} + f_{i+1}^{\text{top}}) = F_{i+1} - F_i \quad (\text{S7a})$$

$$\chi \frac{d\mathcal{L}(f_i^{\text{bot}})}{dt} - (f_{i-1}^{\text{bot}} - 2f_i^{\text{bot}} + f_{i+1}^{\text{bot}}) = F_i - F_{i+1}. \quad (\text{S7b})$$

We now assume that filaments respond symmetrically to stresses, *i.e.*, that they respond to compressive and extensile forces of identical magnitudes by equal and opposite deformations. This is equivalent to considering that  $\mathcal{L}(f)$  is an odd function of  $f$ :

$$\mathcal{L}(f) = -\mathcal{L}(-f). \quad (\text{S8})$$

This condition is fulfilled, *e.g.*, when the filaments are weakly deformed; the relevance of this regime is discussed in detail in the next section. Using Eq. (S8), we find that Eqs. (S7a) and (S7b) can be written as two identical systems of ordinary differential equations for  $f_i^{\text{top}}$  and  $-f_i^{\text{bot}}$ , respectively. As  $f_i^{\text{top}}$  and  $-f_i^{\text{bot}}$  also satisfy identical initial and boundary conditions [Eq. (S2)], we conclude that

$$f_i^{\text{top}} = -f_i^{\text{bot}}. \quad (\text{S9})$$

Inserting this into Eq. (S3), we find  $f_i^{\text{ext}} = 0$ , and therefore the bundle is not contractile. This situation is in contrast with that of Fig. 2(d) of the main text, where a similar bundle exhibits strong contractility as a consequence of violating Eq. (S8).

We thus conclude that both (i) non-identical motors and (ii) an asymmetric elastic response of the filaments are necessary for non-sarcomeric contractility.

## WEAK FILAMENT DEFORMATION AND THE IMMOBILE MOTOR ASSUMPTION

Although the main text deals with the buckling behavior of F-actin, the analysis performed there assumes that filament sections are weakly deformed. Here we recapitulate the points of our model that make use of this assumption, and then justify its use in the frame of our study.

Let us start by considering the analysis of the previous section, which is conducted for an arbitrary force-extension relationship  $\mathcal{L}(f)$  and thus does not suppose small deformation. We now make the assumption that the forces inside the bundle are smaller than the typical force scale  $F_B$  over which the function  $\mathcal{L}$  varies, where  $F_B$  is the filament buckling force [7]. The most obvious consequence is that the force-extension relationships Eqs. (S4) can be linearized according to

$$\mathcal{L}(f) \simeq -cf, \quad (\text{S10})$$

which involves a filament compliance  $c$  which is the same for compression and extension. Combining Eqs. (S4) and (S10) then naturally lead to Eq. (1) of the main text. This straightforward expansion has a less obvious implication: that the motors are immobile throughout the bundle dynamics. Indeed, Eq. (S10) satisfies the condition Eq. (S8), which implies that motors in a complete bundle do not move relative to each other. As long as the bundle stays weakly deformed, it is thus legitimate to represent the motors surrounding a filament of interest as bound to a static effective medium, as shown in Fig. 3(b) of the main text.

To understand how studying a weakly deformed filament can help us understand buckling, we point out that we are only interested in identifying the *onset* of buckling in our bundles. Once buckling sets in, contraction follows according to the simple picture given in Fig. 2(d) of the main text. In that sense, our theoretical approach is akin to a stability analysis of the bundle: we assume that  $f \ll F_B$ , and investigate the conditions under which this assumption breaks down. To the extent that we are not worried about numerical factors of order one, applying the simple buckling criterion  $f > F_B$  to the weakly deformed bundle allows us to formulate predictions for the buckling threshold while keeping our formalism simple.

## DISCUSSION OF THE MOTOR ATTACHMENT-DETACHMENT DYNAMICS

Here we quantitatively justify the picture of the motor attachment-detachment dynamics given in the main text. First, we discuss the assumption that a motor detachment event lasts much less than  $\tau_r$  and  $\tau_d$ , yet is long enough to allow for force relaxation along the bundle. Second, we use known rate constants for the myosin mechanochemical cycle to calculate the value  $\tau_d \approx 200$  ms given in the main text. Third, we justify our assumption that a motor bound to several F-actin sometimes detaches from one of them, but that the probability of simultaneous detachment from several filaments is negligible. Finally, we discuss the possibility that transient binding of the motors to the filament barbed end could play a significant role in bundle contraction, as previously proposed in the theoretical literature [8–12].

### Duration of a detachment event

Consider a thick filament bound to several F-actin, and assume that it detaches from one of them. Here we estimate the time it takes to reattach. Given the high cross-linking of the bundles studied here, the detached F-actin is constrained to stay within a few tens of nanometers of the thick filament, which results in a local

actin concentration of several mM. A coarse approximation of the motor reattachment time  $\tau_{\text{reatt}}$  is obtained by multiplying this concentration with the motor binding rate ( $1.24 \mu\text{M}^{-1} \cdot \text{s}^{-1}$  according to Ref. [13]), giving  $\tau_{\text{reatt}} \approx 1$  ms. This value is consistent with those used in previous models, *e.g.*, Ref. [14].

This reattachment time is negligible compared to the filament relaxation time scale  $\tau_r$ , which ranges from a few tens of milliseconds to several tens of seconds for the motor spacings considered in Fig. 1(f) of the main text. It is also much smaller than the inverse detachment rate  $\tau_d \approx 200$  ms as assumed in the main text. Finally, considering that motors move at a velocity of order  $200 \text{ nm} \cdot \text{s}^{-1}$  as in the main text, the relative motion between motors in the duration of a detachment event is of the order of a fraction of nanometer, *i.e.*, is negligible. Thus we are justified in neglecting the shift of a fast motor relative to its neighbors during a detachment event.

Finally, we consider the case where a force imbalance is present between the two filament sections flanking a motor. If the motor detaches, this force imbalance quickly relaxes. Here we estimate this relaxation time scale. The driving force of the relaxation is filament tension  $f \approx 1$  pN. The friction coefficient between the relaxing filament sections and the rest of the bundle is estimated by considering a rod of length  $L = 1 \mu\text{m}$  undergoing longitudinal translation in a cylinder of radius  $d = 50$  nm (the typical spacing between two filaments) filled with water of viscosity  $\eta$ . The resulting friction coefficient is  $\gamma \approx \eta L$ , yielding a typical relaxation velocity  $v_r = f/\eta L$ . Given that the strain to be relaxed is of the order of a few percent, the typical relaxation length is  $L/100$  and the typical relaxation time is  $(L/100)/v_r = \eta L^2/100f \approx 10 \mu\text{s}$ . This relaxation time scale is much smaller than the duration of a detachment event, and it is thus legitimate to assume that filament stresses fully relax during the course of such an event.

### Frequency of the detachment events

We consider a myosin thick filament bound to an F-actin, and ask how much time it typically takes to detach. Each of our thick filaments typically has 200 heads, and thus  $\approx 100$  heads are facing the actin filament and can potentially bind to it. However, the specifics of the smooth muscle myosin mechanochemical cycle imply that each of these heads spends most of its time—about 96%—detached from the filaments [13]. As a consequence, there is a probability  $P_d = (0.96)^{100} \simeq 0.015$  that all heads are detached at any instant, *i.e.*, that the thick filament is detached from the F-actin of interest.

We next estimate the typical correlation time of the number of heads bound to the F-actin. To do this, we evaluate the typical lifetime of a single myosin-actin bond. According to Ref. [13], a freshly bound myosin

head undergoes two chemical steps leading to dissociation: ATP binding with a rate  $0.47 \mu\text{M} \cdot \text{s}^{-1} \times [\text{ATP}]$  and ATP-induced dissociation with a rate  $1300 \text{s}^{-1}$ . The ATP concentration in our experiments is  $[\text{ATP}] = 1 \text{mM}$ , implying that the mean durations of these steps are 2 ms and 1 ms, respectively. This yields an actomyosin bond lifetime  $\tau_b \simeq 3 \text{ms}$ . As a consequence, time can be divided into intervals of length  $\tau_b$  within which the number of heads bound to the F-actin is typically constant, while the number of heads bound in two consecutive time intervals are independent random variables. As the probability for the thick filament to be detached within each time interval is  $P_d$ , the average time between two detachment events is  $\tau_d = \tau_b/P_d \simeq 200 \text{ms}$ . This is the value we use in the main text.

### Partial vs. complete motor detachment

We now consider a myosin thick filament within a bundle. Given that the cross-section of one of our bundles comprises 4-6 F-actin, we estimate that each myosin thick filament is within binding distance of three or more F-actin. While we established in the previous paragraph that unbinding from each one of these F-actin (partial detachment) occurs frequently, the probability that the thick filament is detached from all of them at any given time is of order  $P_d^3$ . Using the same reasoning as above, this implies that the typical time needed for a thick filament to undergo total detachment is of order  $\tau_b/P_d^3 \approx 1000 \text{s}$ . Thus such events can be neglected on the time scales  $\approx 10 \text{s}$  considered in our study.

Experimentally, we observe that some of the motors unbind from the bundle very quickly ( $< 1 \text{s}$ ) after ATP addition; these are likely weakly bound motors, *e.g.*, motors bound to only one F-actin [1]. Following this fast initial loss of motors, no motor detachment is observed on the typical contraction time scales (a few tens of seconds). These observations support our assumption that motors bound to several F-actin do not undergo total detachment.

### Binding of the motors to the filament barbed ends

Several previous studies assume that motors remain stationary for a finite time upon reaching the barbed end of an F-actin [8–12]. These motors transiently play the role of passive cross-linkers localized at the barbed ends of the filaments, which enables contraction in a sarcomere-like fashion [6]. Here we estimate the amount of barbed-end binding necessary for this effect to play a significant role in our experiments.

Let us consider an actomyosin bundle where the filament barbed ends are occupied by immobilized motors a fraction  $\phi$  of the time. If  $\phi = 1$ , the bundle acts as

a completely sarcomeric bundle. Denoting by  $v$  the velocity of a motor relative to the F-actin and by  $L$  the filament length, each sarcomere contracts with velocity  $2v$  and has length  $2L$ , yielding a strain rate  $v/L$  [see Fig. 1(a) of the main text]. If  $\phi$  is smaller than one, only a fraction of order  $\phi$  of the bundle behaves like a sarcomere, yielding a strain rate  $\phi v/L$  in the absence of externally applied forces. Our experiments are characterized by  $v = 200 \text{nm} \cdot \text{s}^{-1}$  and  $L = 5 \mu\text{m}$ , and thus  $v/L = 0.04 \text{s}^{-1}$ . The bundles considered in the main text are bound to polystyrene beads, which tends to slow their contraction dynamics. We thus consider the results of Ref. [1], where bundles free of such external influences contract with strain rates of the order of  $0.04 \text{s}^{-1}$ . For barbed end binding to significantly contribute to contraction thus requires  $\phi \simeq 1$ , *i.e.*, that each barbed end in the bundle is occupied by a transiently immobilized motor  $\simeq 100\%$  of the time.

As each F-actin is decorated with motors throughout its length, this permanent cross-linking need not be provided by a single motor. Instead, each transiently cross-linked motor needs to stay bound to the barbed end just long enough to be replaced by another incoming motor located further down the same F-actin. As the spacing between two motors is of order  $1 \mu\text{m}$  in this system and the motor velocity is  $200 \text{nm} \cdot \text{s}^{-1}$ , this implies that the typical attachment time of a motor to the filament barbed ends needs to be of order 5 s to account for the observed contraction rate. If such transient binding occurred in actomyosin systems, it would be directly observable. However, we are not aware of an experimental reference reporting such an observation.

### TIME EVOLUTION OF THE FILAMENT FORCE

Using Eqs. (1), (2) and (4) of the main text, we consider the change in the force  $f_i$  over the time interval  $[t, t + dt]$  to first order in  $dt$ . In the absence of any detachment event in motors  $i$  or  $i + 1$  during that time (which happens with probability  $1 - 2dt/\tau_d$ ), we find:

$$f_i(t+dt) = f_i(t) + \frac{dt}{2\tau_r} [f_{i-1}(t) - 2f_i(t) + f_{i+1}(t) + F_{i+1} - F_i], \quad (\text{S11a})$$

which describes a diffusive relaxation of the force in the presence of a source term proportional to  $F_{i+1} - F_i$ . If detachment does occur, then

$$f_i(t+dt) = \frac{f_{i-1}(t) + f_i(t)}{2} \quad (\text{S11b})$$

$$f_i(t+dt) = \frac{f_i(t) + f_{i+1}(t)}{2}, \quad (\text{S11c})$$

where motor  $i$  and  $i + 1$  each detach between  $t$  and  $t + dt$  with probability  $dt/\tau_d$ , as described in Eqs. (S11b) and Eq. (S11c), respectively.

In order to compute  $\langle f \rangle$  and  $\langle f^2 \rangle$ , we need to concern ourselves with both the first and second moments of the force  $f_i$ . Using Eqs. (S11) and denoting the average over detachment events by  $\langle \dots \rangle$ , we obtain

$$\frac{d\langle f_i \rangle}{dt} = \left( \frac{1}{2\tau_r} + \frac{1}{2\tau_d} \right) \langle f_{i-1} - 2f_i + f_{i+1} \rangle + \frac{F_{i+1} - F_i}{\tau_r} \quad (\text{S12a})$$

$$\begin{aligned} \frac{d\langle f_i^2 \rangle}{dt} = & \left( \frac{1}{\tau_r} + \frac{1}{2\tau_d} \right) \langle f_i(f_{i-1} - 2f_i + f_{i+1}) \rangle \\ & + \frac{1}{4\tau_d} \langle f_{i-1}^2 - 2f_i^2 + f_{i+1}^2 \rangle \\ & + \frac{F_{i+1} - F_i}{\tau_r} \langle f_i \rangle \end{aligned} \quad (\text{S12b})$$

$$\begin{aligned} \frac{d\langle f_i f_{i-1} \rangle}{dt} = & - \left( \frac{2}{\tau_r} + \frac{3}{2\tau_d} \right) \langle f_i f_{i-1} \rangle \\ & + \left( \frac{1}{2\tau_r} + \frac{1}{2\tau_d} \right) \langle f_i f_{i-2} + f_{i+1} f_{i-1} \rangle \\ & + \left( \frac{1}{2\tau_r} + \frac{1}{4\tau_d} \right) \langle f_i^2 + f_{i-1}^2 \rangle \\ & + \frac{F_i - F_{i-1}}{\tau_r} \langle f_i \rangle + \frac{F_{i+1} - F_i}{\tau_r} \langle f_{i-1} \rangle \end{aligned} \quad (\text{S12c})$$

$$\begin{aligned} \frac{d\langle f_i f_j \rangle}{dt} = & \left( \frac{1}{2\tau_r} + \frac{1}{2\tau_d} \right) \langle f_i(f_{j-1} - 2f_j + f_{j+1}) \rangle \\ & + \left( \frac{1}{2\tau_r} + \frac{1}{2\tau_d} \right) \langle f_j(f_{i-1} - 2f_i + f_{i+1}) \rangle \\ & + \frac{F_{j+1} - F_j}{\tau_r} \langle f_i \rangle + \frac{F_{i+1} - F_i}{\tau_r} \langle f_j \rangle, \end{aligned} \quad (\text{S12d})$$

where the last equation assumes  $|i - j| \geq 2$  and periodic boundary conditions are used for simplicity.

The continuum limit of Eq. (S12a) leads to Eq. (5) of the main text, which describes the evolution of the first moment of the filament tension  $f(x, t)$ . A few more steps are necessary to obtain the equations for the second moments. Denoting  $N = \ell_f/\ell_0$ , we introduce the spatial correlation functions

$$U_i = \sum_{j=1}^N \overline{\langle f_j f_{j+i} \rangle} \quad (\text{S13a})$$

$$V_i = \sum_{j=1}^N \overline{\langle f_j \rangle F_{j+i}}, \quad (\text{S13b})$$

where  $\overline{\dots}$  denotes averaging over the random motor distribution. Combining these definitions with Eqs. (S12) and the initial condition  $f_i(t=0) = 0$ , we find the symmetry relations

$$U_i = U_{-i} \quad \text{and} \quad V_i = -V_{1-i}, \quad (\text{S14})$$

which we use along with Eqs. (S12) to derive the evolution equations

$$\begin{aligned} \partial_t U_i = & \left[ \left( \frac{2D}{\ell_0^2} + \frac{\delta_{i,1} + \delta_{i,0}}{2\tau_r} \right) (U_{i-1} - U_i) \right. \\ & \left. + \left( \frac{2D}{\ell_0^2} + \frac{\delta_{i,-1} + \delta_{i,0}}{2\tau_r} \right) (U_{i+1} - U_i) \right] + \frac{V_{i+1} - V_i}{\tau_r} \end{aligned} \quad (\text{S15a})$$

$$\partial_t V_i = \frac{2D}{\ell_0^2} (V_{i-1} - 2V_i + V_{i+1}) + \frac{N\delta F_S^2}{2\tau_r} (\delta_{i,1} - \delta_{i,0}), \quad (\text{S15b})$$

where  $D$ ,  $\ell_0$  and  $\delta F_S$  are defined as in the main text and  $\delta_{i,j}$  is the Kronecker delta. To leading order in  $\ell_0$ , the continuum limit  $i \rightarrow x/\ell_0$  yields

$$\partial_t U = 2D\partial_x^2 U + (\ell_0/\tau_r)\partial_x V \quad (\text{S16a})$$

$$\partial_t V = 2D\partial_x^2 V - (N\ell_0^2\delta F_S^2/2\tau_r)\partial_x [\delta(x)], \quad (\text{S16b})$$

where  $\delta(x)$  is the Dirac delta function. Note that as  $f_{i+1} - f_i \rightarrow \ell_0\partial_x f$  and  $\delta_i \rightarrow \ell_0\delta(x)$  in the continuum limit, the sum of the terms involving the Kronecker deltas in Eq. (S15a) is of order  $\ell_0\partial_x[\ell_0\delta(x)\ell_0\partial_x U] \propto \ell_0^3$ . This expression is of order three in  $\ell_0/\ell_f$ , and can thus be neglected compared to the sum of the terms proportional to  $D$ , which is of order two. Solving for  $V$ , then  $U$  in Fourier space, we find

$$U(x, t) = Nf_\infty^2 \sum_{n \in \mathbb{Z}^*} \left[ \frac{3e^{2i\pi nx/\ell_f}}{n^2\pi^2} \left( 1 - e^{-\frac{n^2 D t}{(2\pi\ell_f)^2}} \right)^2 \right], \quad (\text{S17})$$

where  $f_\infty$  is given in Eq. (6) of the main text. Taking the  $x \rightarrow 0$  limit of this expression, we find

$$\overline{\langle f^2 \rangle}(t) = U(0, t)/N = f_\infty^2 \sum_{n \in \mathbb{Z}^*} \left[ \frac{3}{n^2\pi^2} \left( 1 - e^{-\frac{n^2 D t}{(2\pi\ell_f)^2}} \right)^2 \right], \quad (\text{S18})$$

which we plot in Fig. 4(b) of the main text. Note that in the continuum limit used here  $\overline{\langle f^2 \rangle} = \langle f \rangle^2$ . This implies that we can use the behavior of  $\langle f \rangle^2$ , which can be inferred from Eq. (5) of the main text, to understand the behavior of the typical force  $\overline{\langle f^2 \rangle}$ . Indeed, this type of reasoning is implicit in the discussion leading to Eq. (9) of the main text.

### NON-IDENTICAL MOTOR SPACINGS AND FORCE-DEPENDENT FILAMENT DETACHMENT

The model presented in the main text is designed to be as simple as possible while accounting for experimental observations. Namely, we demand that it recapitulate bundle contractility at relatively high myosin concentration, and the absence of contractility at low myosin density. This requires including non-identical motor unloaded velocities and motor detachment in the model.

While these simple features yield good agreement with the experiments, one might wonder how additional features of realistic systems would affect our conclusions. Here we numerically investigate two such features: a distribution of inter-motor distances  $\ell_0$  and the dependence of the motor detachment rate on applied force. We find that neither significantly affects our main results, which confirms that the simple model of the main text captures the essential physics of the system studied.

We solve Eqs. (S11) numerically with finite but small  $dt$  for an array of  $N = 10$  motors. If the motor stall forces are all identical (*i.e.*,  $\delta F_S = 0$ ), force build-up within the bundle does not occur, thus preventing contraction. Instead, we choose the motor stall forces at random from a distribution with significant spread, *i.e.*, one whose standard deviation is comparable to its mean. We thus pick stall forces from a homogeneous distribution between 0 and  $2F_S$  (thus  $\delta F_S = F_S/\sqrt{3}$ ). We do not expect our results to strongly depend on the precise form of this distribution. We start the simulations with a relaxed bundle ( $f_i = 0$ ) and run them long enough to reach a steady state for  $\sum_{i=1}^N f_i^2$ . Here we present results for  $f_\infty^2 = \lim_{t \rightarrow \infty} \langle f^2 \rangle$ . All values of  $f_\infty$  presented here are averaged over 100 independent realizations of the system, each with a different set of motor stall forces, as well as motor spacings when appropriate. The steady-state force in each realization is averaged over time after the simulation reaches its steady state.

To study the effect of a distribution of inter-motor distances  $\ell_0$ , we compare the case where  $\ell_0 = \ell_0^{\text{avg}}$  everywhere with a situation where  $\ell_0$  is homogeneously distributed in the interval

$$\ell_0^{\text{avg}}/2 < \ell_0 < 3\ell_0^{\text{avg}}/2. \quad (\text{S19})$$

This distribution is chosen for its significant spread and the fact that it avoids numerical convergence issues due to very small values of  $\ell_0$ . Again, we do not expect our results to strongly depend on the precise form of this distribution. As shown by the dashed line in Fig. S3, we find that the relationship between the steady state force  $f_\infty$  and the motor detachment time  $\tau_d$  is qualitatively similar to that given by the analytical solution of the main text [Eq. (6)—see Fig. S3, solid line]. The distribution of  $\ell_0$  results in a horizontal shift of the curve by a factor of order one, an effect that is unimportant for the scaling analysis of the main text.

To study the effect of force-dependent motor detachment, we assume that the rate of motor detachment depends on the force exerted by the filament on the motor. Experiments performed with smooth muscle myosin indicate that a motor detaches less frequently (more frequently) when the exerted force opposes (assists) its natural motion, a tendency known as the Fenn effect [15]. These observations suggest an exponential dependence

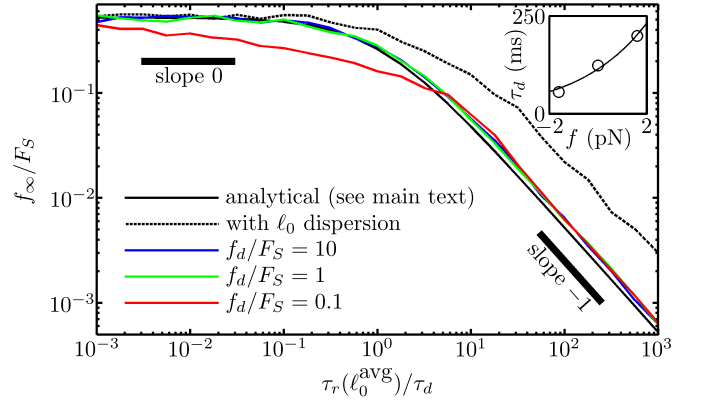

FIG. S3. Effect of inhomogeneous inter-motor spacings and force-dependent motor detachment on the steady-state filament force. The typical steady-state filament force  $f_\infty$  is plotted as a function of the dimensionless unloaded detachment rate  $\tau_r/\tau_d$ . Two asymptotic behaviors identical to those apparent in Fig. 4 of the main text are observed. Little difference is observed between the calculation of the main text [solid black line—Eq. (6)], the case with inhomogeneous inter-motor spacing  $\ell_0$  [dashed line—see Eq. (S19)], and the case with force-dependent motor detachment [colored lines—see Eq. (S20)]. Inset: Fit of the relationship Eq. (S20) to the data of Ref. [15], yielding  $f_d \simeq 2.8$  pN.

for the rate of detachment of motor  $i$ :

$$\frac{1}{\tau_d} \exp\left(\frac{f_i - f_{i-1}}{f_d}\right) \quad (\text{S20})$$

As shown in the inset of Fig. S3, this dependence involves a typical force  $f_d \simeq 2.8$  pN. We plot the resulting dependence of the typical filament force  $f_\infty$  on the dimensionless unloaded detachment rate  $\tau_r/\tau_d$  for different values of  $f_d$  in Fig. S3. Since  $f_d$  and  $F_S$  are both expected to be  $\approx$  pN, we show three curves covering the range of realistic ratios  $f_d/F_S = 10, 1$  and  $0.1$ . The two first curves are found to be very close to the result of the main text (corresponding to  $f_d = \infty$ ), while third one differs from it by a factor of order one at most.

Taken together, the results of this section indicate that neither a distribution of inter-motor spacing nor a force-dependent detachment rate have a strong influence on the results presented in the main text. This thus validates our simplifying assumptions of constant  $\ell_0$  and  $\tau_d$  in the frame in our scaling/order-of-magnitude approach.

## SUPPLEMENTAL MOVIE LEGENDS

- **Movie S1:** Myosin density dependence of reconstituted actomyosin bundle contraction. Inverted contrast time-lapse images of Oregon Green myosin in bundles with  $\ell_0 = 540$  nm (*left*) or  $1.5 \mu\text{m}$  (*right*). 1 mM ATP is added at  $t = 0$  s. For  $\ell_0 = 540$  nm,

the bends within the bundle straighten out quickly and the bundle becomes taut within 15 s of ATP addition while the bundle with  $\ell_0 = 1.5 \mu\text{m}$  remains floppy and bent.

- **Movie S2:** F-actin buckling during contraction. Inverted contrast time-lapse images of Oregon Green myosin (*left*) and Alexa 568-phalloidin-stabilized F-actin (*right*) shown in Fig. 2(c) of the main text. Contraction is initiated by the addition of 1 mM ATP at  $t = 0$  s. Arrows indicate buckling events. Bar,  $5 \mu\text{m}$ .

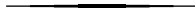

- [1] T. Thoresen, M. Lenz, and M. L. Gardel. Reconstitution of contractile actomyosin bundles. *Biophys. J.*, 100(11):2698, 2011.
- [2] M. Lenz and A. Dinner. Requirements for disordered actomyosin bundle contractility. arXiv:1101.1058, 2011.
- [3] A. Carvalho, A. Desai, and K. Oegema. Structural memory in the contractile ring makes the duration of cytokinesis independent of cell size. *Cell*, 137(5):926, 2009.
- [4] W. M. Bement and D. G. Capco. Analysis of inducible contractile rings suggests a role for protein kinase C in embryonic cytokinesis and wound healing. *Cell Motil. Cytoskeleton*, 20(2):145, 1991.
- [5] A. M. Herrera, B. E. McParland, A. Bienkowska, R. Tait, P. D. Paré, and C. Y. Seow. “sarcomeres” of smooth muscle: functional characteristics and ultrastructural evidence. *J. Cell Sci.*, 118(11):2381, 2005.
- [6] A. Zemel and A. Mogilner. Motor-induced sliding of microtubule and actin bundles. *Phys. Chem. Chem. Phys.*, 11(24):4821, 2009.
- [7] T. Odijk. Stiff chains and filaments under tension. *Macromolecules*, 28(20):7016, 1995.
- [8] K. Kruse and F. Jülicher. Actively contracting bundles of polar filaments. *Phys. Rev. Lett.*, 85(8):1778, 2000.
- [9] K. Kruse and K. Sekimoto. Growth of fingerlike protrusions driven by molecular motors. *Phys. Rev. E*, 66(3):031904, 2002.
- [10] K. Kruse and F. Jülicher. Self-organization and mechanical properties of active filament bundles. *Phys. Rev. E*, 67(5):051913, 2003.
- [11] T. B. Liverpool and M. C. Marchetti. Instabilities of isotropic solutions of active polar filaments. *Phys. Rev. Lett.*, 90(13):138102, 2003.
- [12] R. Peter, V. Schaller, F. Ziebert, and W. Zimmermann. Pattern formation in active cytoskeletal networks. *New J. Phys.*, 10(3):035002, 2008.
- [13] S. S. Rosenfeld, J. Xing, L.-Q. Chen, and H. L. Sweeney. Myosin IIB is unconventionally conventional. *J. Biol. Chem.*, 278(30):27449, 2003.
- [14] B. Gilboa, David Gillo, O. Farago and A. Bernheim-Groswasser. Bidirectional cooperative motion of myosin-II motors on actin tracks with randomly alternating polarities. *Soft Matter*, 5(11):2223–2231, June 2009.
- [15] C. Veigel, J. E. Molloy, S. Schmitz, and J. Kendrick-Jones. Load-dependent kinetics of force production by smooth muscle myosin measured with optical tweezers. *Nat. Cell Biol.*, 5(11):980, 2003.
